# Supplementary material for: DualEquiNet: A Dual-Space Hierarchical Equivariant Network for Large Biomolecules
Source: arXiv:2506.19862 source file (2025-06-10)
Supplement: Supplementary file 1 [file proofs.tex]

\section{Proof of Equivariance}
\label{appen:proofs}

In this section, we formally show the equivariance property of our proposed DualEqui model. Specifically, we commence by introducing the basic notations and facts used in this section in Section~\ref{appen:proofs_prelim}. Next, we first show the invariance property of basic message functions in Section~\ref{appen:proofs_msg_func}, and then show the equivariance property of the entire model in Section~\ref{appen:proofs_entire_model}.

\subsection{Preliminaries}\label{appen:proofs_prelim}

In this proof, we aim at showing DualEqui is E(3)-equivariance to a combination of rotation and translation, where we impose the rotation matrix $R_\theta \in \mathbb{R}^{3\times3}$ and the translation vector $t\in\mathbb{R}^3$ imposed on the input 3D coordinates of atoms $\boldsymbol{x}_i\in\mathbb{R}^3,i\in\{1,\ldots,N\}$. 

For notation convenience, we let $z$ be an arbitrary intermediate variable in our model computation (e.g., message $m_{E,ij}$ in Eq.~\eqref{eq:eu_space_msg}), we sometimes abuse its notation in a functional form, writing it as a function of its related variables, such as $z(\boldsymbol{x}_{ij})$ or $z(\hat{\boldsymbol{x}}_{i})$. This allows us to denote the model output under E(3) transformations as $z(R_\theta\boldsymbol{x}_{ij}+t)$, and check whether equivariance or invariance holds. By default, we regard the original non-function form intermediate variables $z$ as a shorthand notation for $z(R_\theta\boldsymbol{x}_{ij}+t)$, where $R_\theta = I$ and $t=0$.

%we use ... (introduce the "function" notation system)

We first introduce some important basic facts, which is useful for further proof in this paper.

\begin{lemma}[Invariance of the Euclidean Distance]\label{lem:eqvar_l2}
    For any pair of 3D coordinate vectors $\boldsymbol{x}_i,\boldsymbol{x}_j \in \mathbb{R}^3$, the Euclidean distance $\| \boldsymbol{x}_i - \boldsymbol{x}_j \|$ is invariant to E(3) transformations. 
    %For any pair of relative position vector $\boldsymbol{x}_i,\boldsymbol{x}_j \in \mathbb{R}^3$ and E(3) transformation characterized by rotation matrix $R_\theta \in \mathbb{R}^3$ and translation vector $t \in \mathbb{R}^3$, we have $\| \boldsymbol{x}_{ij} \|_ = \| R_\theta \boldsymbol{x}_{ij} + t\|$, where $\boldsymbol{x}_{ij} =\boldsymbol{x}_i - \boldsymbol{x}_j$. 
\end{lemma}
\begin{proof}
    Let the E(3) transformation be characterized by rotation matrix $R_\theta \in \mathbb{R}^{3\times3}$ and translation vector $t \in \mathbb{R}^3$. Applying the transformation to both $\boldsymbol{x}_i$ and $\boldsymbol{x}_j$, we can conclude by basic algebra that:
    \begin{align*}
        \| (R_\theta \boldsymbol{x}_i + t) - (R_\theta \boldsymbol{x}_j + t) \| = & ~ \| R_\theta (\boldsymbol{x_i} - \boldsymbol{x}_j) \| \\
        & = ~ \sqrt{(\boldsymbol{x_i} - \boldsymbol{x}_j)^\top R_\theta^\top \cdot R_\theta (\boldsymbol{x_i} - \boldsymbol{x}_j)} \\
        & = \| \boldsymbol{x_i} - \boldsymbol{x}_j\|,
    \end{align*}
    which completes the proof.

    % Since we have
    % \begin{align*}
    %     \| R_\theta x\| = & ~ \sqrt{ (\boldsymbol{x}^\top R_\theta^\top) \cdot (R_\theta \boldsymbol{x})} \\ 
    %     & = ~ \sqrt{\boldsymbol{x}^\top \boldsymbol{x}} \\ 
    %     & = ~ \| \boldsymbol{x} \|.
    % \end{align*}
    % where the first and the last step follow from the definition of $\ell_2$ norm, and the second step follows from the fact that $R_\theta^\top R_\theta=I$. 

    % The proof is complete.
\end{proof}

\begin{lemma}[Equivariance of the Unit Direction Vector]\label{lem:eqvar_unit}
     For any pair of 3D coordinate vectors $\boldsymbol{x}_i,\boldsymbol{x}_j \in \mathbb{R}^{3\times 3}$, the unit direction vector $\hat{\boldsymbol{x}}_{ij}:=\boldsymbol{x}_{ij}/\|\boldsymbol{x}_{ij}\|$ is equivariant to E(3) transformations. 
\end{lemma}
\begin{proof}
    Let the E(3) transformation be characterized by rotation matrix $R_\theta \in \mathbb{R}^3$ and translation vector $t \in \mathbb{R}^3$. Since Euclidean distance is invariant by Lemma~\ref{lem:eqvar_l2}, applying the transformation to both $\boldsymbol{x}_i$ and $\boldsymbol{x}_j$ yields
    \begin{align*}
        \hat{\boldsymbol{x}}_{ij}(R_\theta\boldsymbol{x}_i+t,R_\theta\boldsymbol{x}_j+t) = & ~ R_\theta\frac{\boldsymbol{x}_{ij}}{\| \boldsymbol{x}_{ij} \|} \\
        = & ~ R_\theta \hat{\boldsymbol{x}}_{i,j}, 
    \end{align*}
    which completes the proof.
\end{proof}

\begin{lemma}[Equivariance of the Spherical Harmonics Features]\label{lem:eqvar_sh_in_prod}
    Any Spherical Harmonics feature $\boldsymbol{r}_{i} \in \mathbb{R}^{2l+1}$ in Eq.~\eqref{eq:init_sh_neigh} is equivariant to E(3) transformations. 
    %Let $r_i, r_j$ be two spherical harmonics features as defined in Eq.~\eqref{eq:init_sh_neigh}. Under any rotation matrix $R_\theta$, we have $r_i(R_\theta) \cdot r_j(R_\theta) = r_i\cdot r_j$. 
\end{lemma}
\begin{proof}
    First, we recall Eq.~\eqref{eq:init_sh_neigh} for the definition of the Spherical Harmonics features:
    \begin{align*}
        \boldsymbol{r}_{i} = \frac{1}{|\mathcal{N}_{E}(i)|} \sum_{j \in \mathcal{N}_{E}(i)} \phi_0 \left( \left[h_i, h_j, \left\|\boldsymbol{x}_{ij} \right\| \right] \right) \  Y\left( \boldsymbol{\hat{x}}_{ij} \right).
    \end{align*}

    Let our E(3) transformation characterized by rotation matrix $R_\theta \in \mathbb{R}^{3\times3}$ and translation vector $t \in \mathbb{R}^3$. Since we can conclude by Lemma~\ref{lem:eqvar_unit} and basic algebra that equivariant variables $\boldsymbol{x}_{ij}$ and $\hat{\boldsymbol{x}}_{ij}$ yields $R_\theta\boldsymbol{x}_{ij}$ and $R_\theta\hat{\boldsymbol{x}}_{ij}$ under the transformation, we can show the equivariance of $\boldsymbol{r}_i$ by:
    \begin{align*}%\label{eq:eqvar_sh_in_prod_step1}
        \boldsymbol{r}_{i}(R_\theta\boldsymbol{x}_i + t, \{j\in\mathcal{N}_E(i):R_\theta\boldsymbol{x}_j+t\}) =& ~\frac{1}{|\mathcal{N}_{E}(i)|} \sum_{j \in \mathcal{N}_{E}(i)} \phi_0 \left( \left[h_i, h_j, \left\|R_\theta\boldsymbol{x}_{ij} \right\| \right] \right) \  Y\left( R_\theta\boldsymbol{\hat{x}}_{ij} \right) \notag \\ 
        = & ~  \frac{1}{|\mathcal{N}_{E}(i)|} \sum_{j \in \mathcal{N}_{E}(i)} \phi_0 \left( \left[h_i, h_j, \left\|\boldsymbol{x}_{ij} \right\| \right] \right) \  Y\left( R_\theta\boldsymbol{\hat{x}}_{ij} \right) \notag \\
        = & ~ \frac{1}{|\mathcal{N}_{E}(i)|} \sum_{j \in \mathcal{N}_{E}(i)} \phi_0 \left( \left[h_i, h_j, \left\|\boldsymbol{x}_{ij} \right\| \right] \right) \  D(R_\theta)Y\left(\boldsymbol{\hat{x}}_{ij} \right) \notag \\
        = & ~ D(R_\theta) \cdot\boldsymbol{r}_i,
    \end{align*}
    where $D(R_0)$ denotes the Wigner-D matrix.
    %where the first step follows from the definition of $r_i$ and basic geometric property, the second step follows from Lemma~\ref{lem:eqvar_l2}, the third step follows from the property of the Wigner-D matrix, and the last step follows from basic algebra. 

    % Therefore, we can further conclude that
    % \begin{align*}
    %     r_i(R_\theta) \cdot r_j(R_\theta) = & ~ r_i(R_\theta)^\top r_j(R_\theta) \\ 
    %     = & ~(r_i^\top D(R_\theta)^\top)\cdot (D(R_\theta) r_j) \\ 
    %     = & ~ r_i^\top r_j \\
    %     = & ~ r_i \cdot r_j,
    % \end{align*}
    % where the first step and the last step follow from the definition of inner product, the second step follows from Eq.~\eqref{eq:eqvar_sh_in_prod_step1}, and the third step follows from the fact that $D(R_\theta)^\top D(R_\theta) =I$. 

    % Thus, the proof is finished. 
\end{proof}    

\subsection{Invariance of Message Functions}\label{appen:proofs_msg_func}

Built upon the previous basic facts on equivariant and invariant quantities, we present the invariance of basic message functions in this paper, including $m_{E, ij}$ and $m_{SH\to E,ij}$ and $m_{E\to SH,ij}$. 

\paragraph{Invariance of $m_{E, ij}$.} Recalling Eq.~\eqref{eq:eu_space_msg}, the message function $m_{E, ij}$ can be written as:
\begin{align*}
    m_{E, ij} = & ~ \phi_{E} \left( \left[h_i, h_j, \left\|\boldsymbol{x}_{ij} \right\| \right] \right).
\end{align*}
Since $h_i$ and $h_j$ are transformation irrelevant scalars and $\| \boldsymbol{x}_{ij} \|$ is invariant as shown in Lemma~\ref{lem:eqvar_l2}, we can conclude that the message function $m_{E, ij}$ is invariant by the fact that it only incoporates invariant quantities for computation.

\paragraph{Invariance of $m_{SH\to E, ij}$.} Let $r_i,r_j$ denote any arbitrary pairs of spherical harmonics features. The following quantity is invariant following the equivariance of spherical harmonics features in Lemma~\ref{lem:eqvar_sh_in_prod}:
\begin{align*}
    r_i \odot r_j  = [\boldsymbol{r}_i^{0}\cdot\boldsymbol{r}_j^{0}, \boldsymbol{r}_i^{1}\cdot\boldsymbol{r}_j^{1}, \cdots, \boldsymbol{r}_i^{l_{max}}\cdot\boldsymbol{r}_j^{l_{max}}].
\end{align*}

Thus, combining with the formulation of $m_{SH\to E, ij}$:
\begin{align*}
    m_{E \to SH, ij} = \psi_{E \to SH} ([r_i \odot r_j, \left\|\boldsymbol{x}_{ij} \right\|]]),
\end{align*}
we can simply conclude that $m_{E \to SH, ij}$ is invariant, since both $r_i \odot r_j$ and $\| \hat{\boldsymbol{x}}_{ij} \|$ are invariant.

\paragraph{Invariance of $m_{SH, ij}$.} Since $r_i \odot r_j$ is an invariant quantity and both $h_i$ and $h_j$ are irrelevant to the transformations, and the $m_{SH, ij}$ can be formulated as follows:
\begin{align*}
    m_{SH, ij} = \phi_{E} \left( \left[h_i, h_j, r_i \odot r_j \right] \right).
\end{align*}

We can simply conclude that $m_{SH, ij}$ is invariant. 

\paragraph{Invariance of $m_{E \to SH, ij}$.}.

\subsection{Equivariance of the DualEqui Model}\label{appen:proofs_entire_model}

\paragraph{Equivariance of Eq.~\ref{eq:delta_h_e} ($\Delta h_{E, i}$)}

    Therefore, the equivariance of $\Delta h_{E, i}$ in Eq.~\eqref{eq:delta_h_e} can be shown as follows:
    \begin{align*}\label{eq:delta_h_e_step2}
        \Delta h_{E, i}(R_\theta) = & ~ \frac{1}{K} \sum_{k=1}^K \phi_{E, h} \left( \left[ h_i, \bigoplus_{j \in \mathcal{N}_{E}(i)} \alpha_{E, ij}^k \ \phi_{E, h}^k (m_{E, ij}(R_\theta)) + \bigoplus_{j \in \mathcal{N}_{SH}(i)} \beta_{E, ij}^k \psi_{E, h}^k (m_{SH \to E, ij}(R_\theta)) \right] \right) \\ 
        = & ~ \frac{1}{K} \sum_{k=1}^K \phi_{E, h} \left( \left[ h_i, \bigoplus_{j \in \mathcal{N}_{E}(i)} \alpha_{E, ij}^k \ \phi_{E, h}^k (m_{E, ij}) + \bigoplus_{j \in \mathcal{N}_{SH}(i)} \beta_{E, ij}^k \psi_{E, h}^k (m_{SH \to E, ij}) \right] \right) \\ 
        = & ~ \Delta h_{E, i},
    \end{align*}
    where the first step follows from the basic geometric property, the second step follows from the equivariance of the message functions in Eq.~\eqref{eq:delta_h_e_step1} and Eq.~\eqref{eq:delta_h_e_step2}, and the last step directly follows from Eq.~\eqref{eq:delta_h_e}. 

    Therefore, we can conclude that $\Delta h_{E, i}$ in Eq.~\eqref{eq:delta_h_e} is equivariant under rotations.

\paragraph{Equivariance of Eq.~\ref{eq:delta_x_e} ($\Delta \boldsymbol{x}_{E, i}$)}
\begin{proof}

\end{proof}

\paragraph{Equivariance of Eq.~\ref{eq:delta_h_sh} ($\Delta h_{SH, i}$)}
% very similar to the first one, only needs to show to message is invariant. Then remaining is similar
\begin{proof}

\end{proof}

\paragraph{Equivariance of Eq.~\ref{eq:delta_r_sh} ($\Delta \boldsymbol{r}_{SH, i}$)}
\begin{proof}

\end{proof}

\paragraph{Equivariance of Eq.~\ref{eq:h_pooling} (Pooling of $h$)}
\begin{proof}

\end{proof}

\paragraph{Equivariance of Eq.~\ref{eq:x_pooling} (Pooling of $\boldsymbol{x}$)}
\begin{proof}

\end{proof}

\paragraph{Equivariance of Eq.~\ref{eq:r_pooling} (Pooling of $\boldsymbol{r}$)}
\begin{proof}

\end{proof}
